# Supplementary material for: DeepSAT: An EDA-Driven Learning Framework for SAT
Source: arXiv:2205.13745 source file (2023-01-20)
Supplement: Supplementary file 1 [file appendix.tex]

% \section{Implementation Details}

% Our code and pre-trained models are available at:\url{}.

\begin{figure}[t!]
	\centering
	\includegraphics[width=0.7\linewidth]{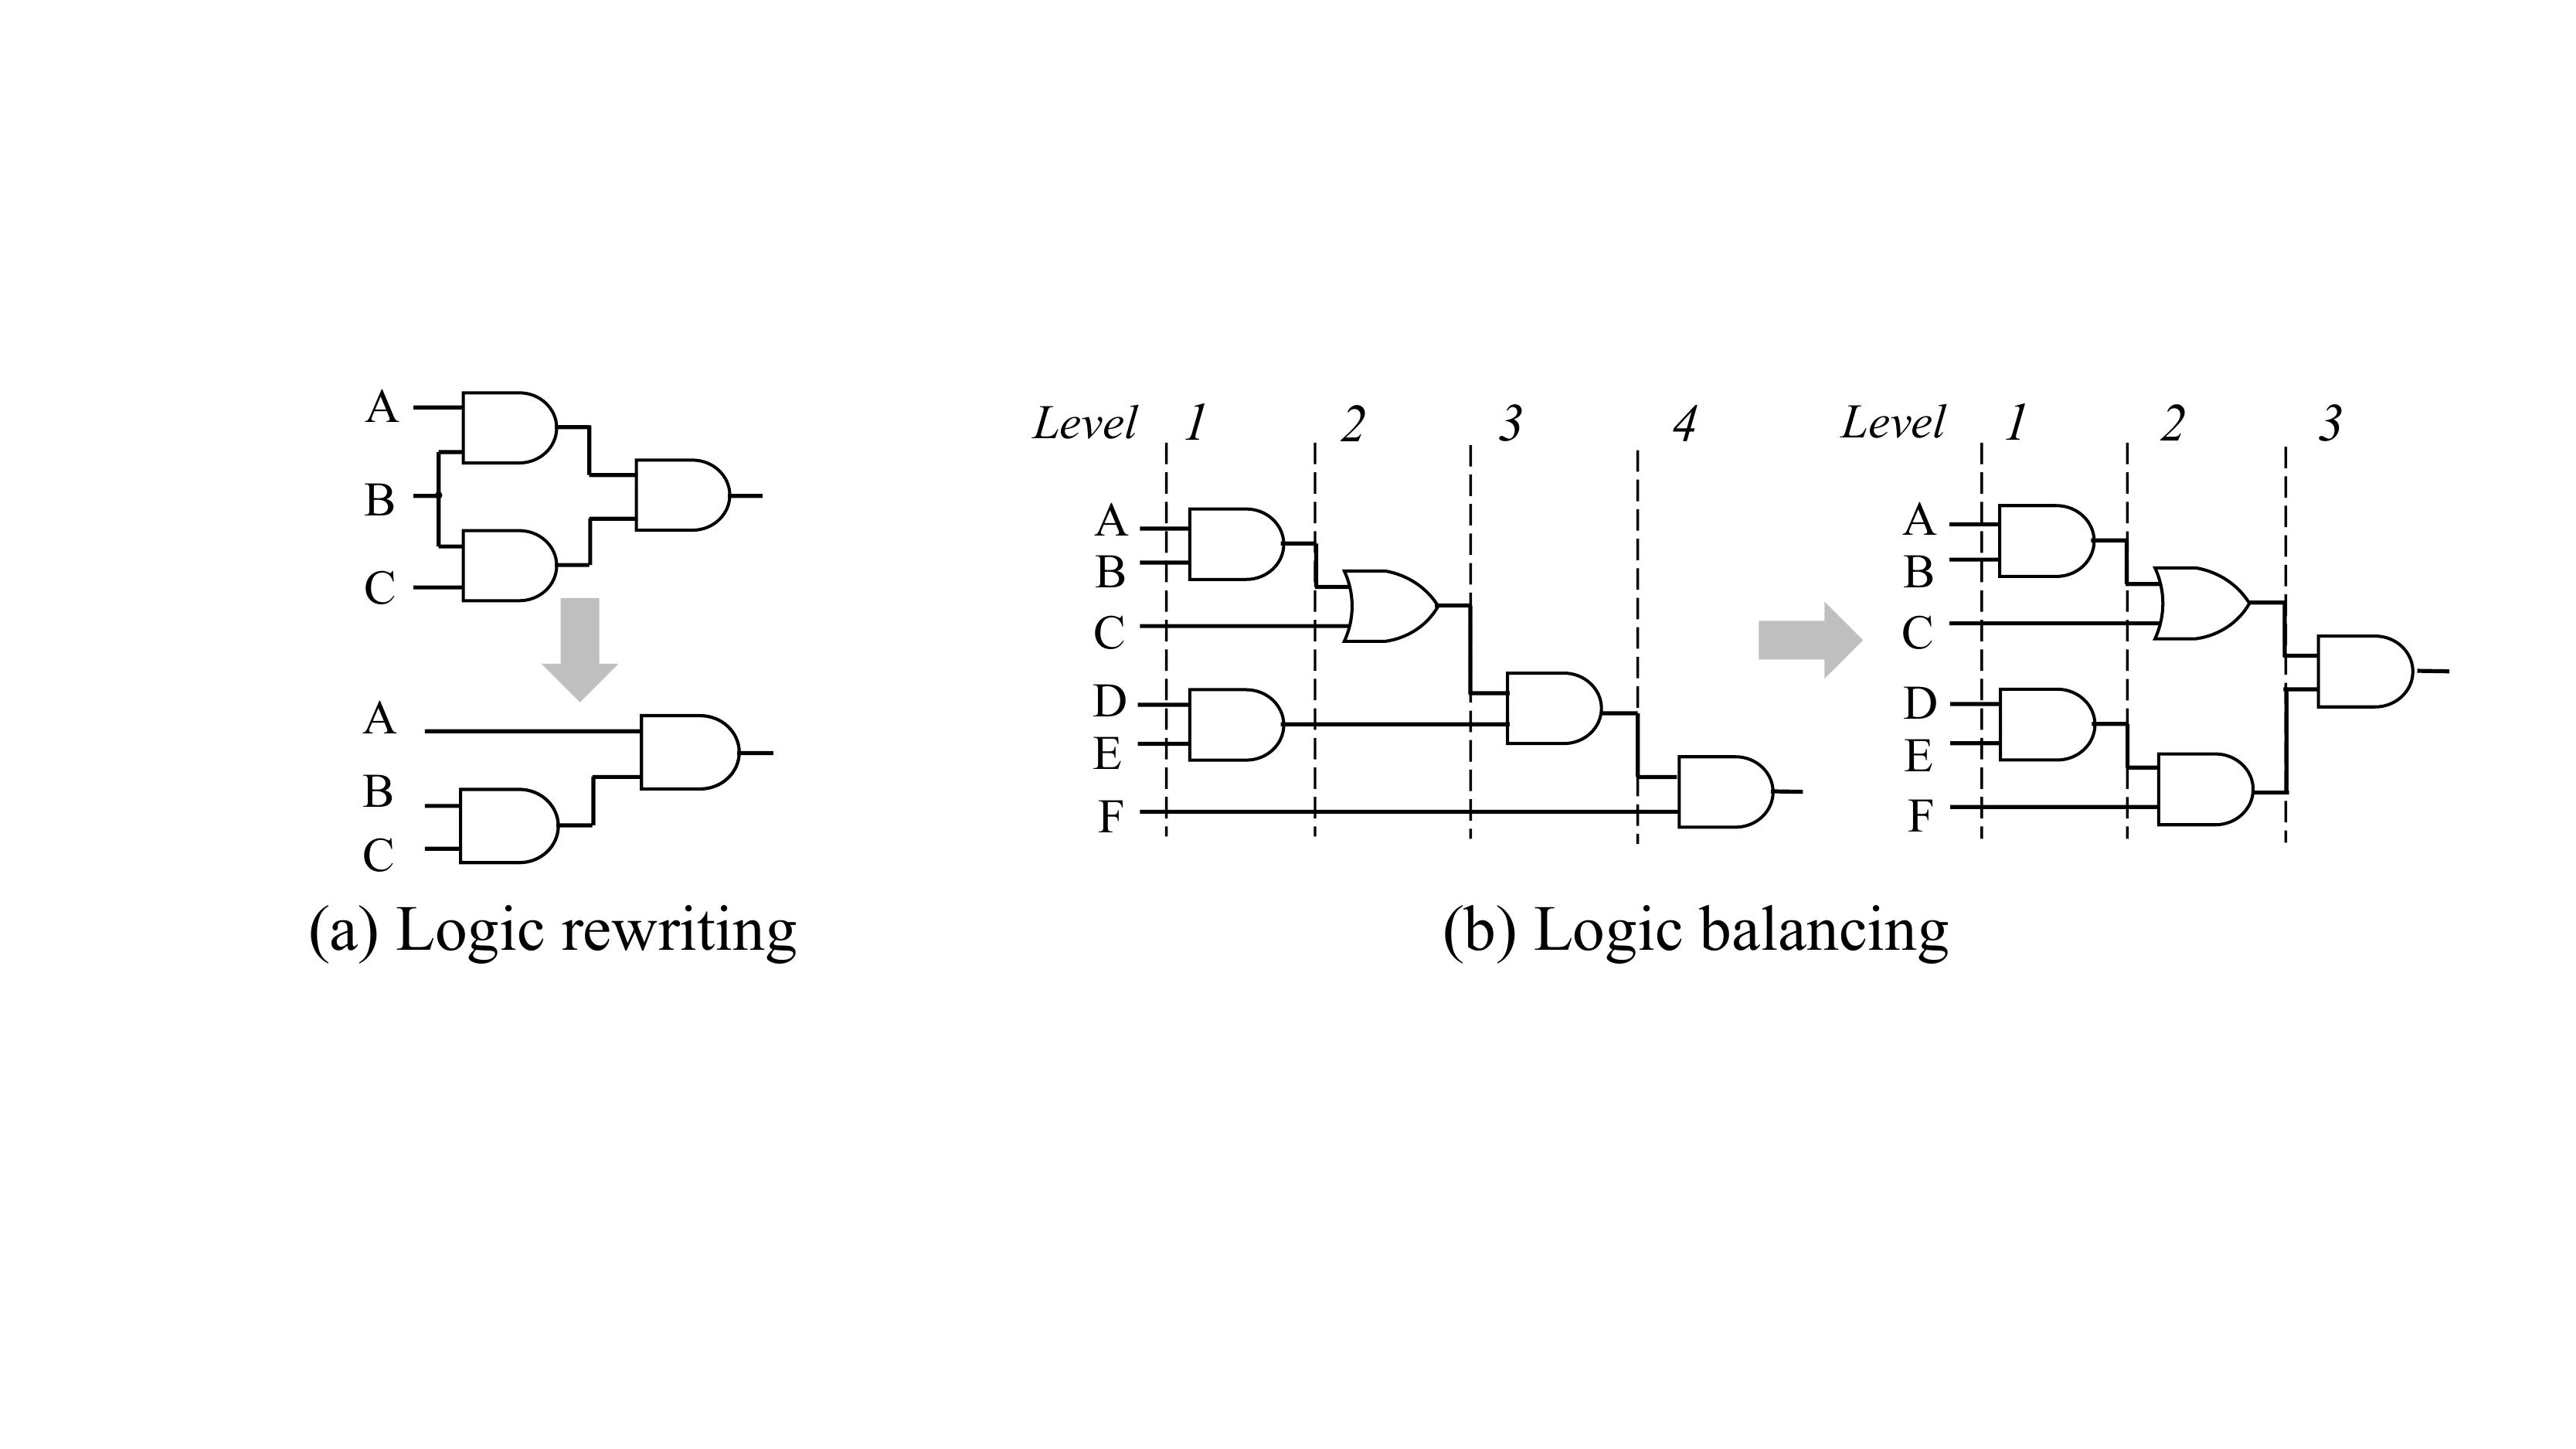}
	\vspace{-10pt}
	\caption{Examples of graph optimization based on logic synthesis.}
	\label{FIG:rwbl}
	\vspace{-10pt}
\end{figure}
\section{Logic Synthesis}\label{appendix:syn}
We apply two techniques of logic synthesis in Section~\ref{subsec:transformation}, namely logic rewriting and logic balancing. In this section, we give more details about these two techniques. Examples of graph optimization based on logic synthesis are included in Figure~\ref{FIG:rwbl}.

\subsection{Logic Rewriting}
Rewriting is a greedy circuit optimization technique for minimizing the circuit structure~\cite{bjesse2004dag, mishchenko2006dag}. It enumerates sub-graphs and replaces them with the equivalent smaller sub-graphs iteratively. To facilitate subsequent discussion, we first define \textit{cut} as a set of nodes on the circuits with only one root node. A cut is \textit{K-feasible} if the number of variables does not exceed $K$. In AIG rewriting~\cite{mishchenko2006dag}, all non-redundant 4-feasible cuts are pre-computed and stored in advance. 
With the above prerequisite, 
the rewriting algorithm can be summarized as the following four steps: (1) select a certain node as the root node in the topological order from PI to PO; (2) perform the 4-feasible cut enumeration; (3) in each iteration, get a cut and corresponding Boolean function; (4) if there is an implementation of the function with a smaller number of gates, choose the implementation; otherwise, leave the AIG unchanged.
Figure~\ref{FIG:rwbl}(a) shows an example where the sub-graph can be replaced by a simplified one without logic modification. 

\subsection{Logic Balancing}
Logic balance creates an equivalent circuit with minimum delay, i.e., the minimum number of logic levels. As suggested by its name, the optimized circuits is derived by balancing the various fan-in regions of multi-input gates. The main algorithm constructs a Boolean function trees and decomposes the tree from root to leaves~\cite{cortadella2003timing}.
In our setting, since all AND gates only have two fan-in wires, the logic balance refers to logic bi-decomposition problem. In each balancing iteration: (1) the logic tree is decomposed into several sub-trees; (2) balance the sub-tree recursively; (3) insert the balanced sub-trees back to the main stem. 
Figure~\ref{FIG:rwbl}(b) shows a logic balancing instance, where the balancing achieves one logic level reduction. 

The above logic synthesis techniques are implemented in the open-source tool ABC~\cite{brayton2010abc} with commands \textit{rewrite / rw} and \textit{balance / b}, respectively. 
It should be noted that both commands achieve the locally optimal effect based on the current topological structure. In other words, the circuit will not be modified when executing the same command  for multiple times. Therefore, including some perturbation into the circuit can expose new minimizing opportunities. For example, \cite{een2007applying} perturbs the AIG by decomposing the local structure and \cite{cortadella2003timing} transforms the circuit based on different laws alternately. The \textit{rewrite} and \textit{balance} operations are considered as perturbation factors mutually. 
In this work, we perform both operations iteratively for three times (\textit{rw; b; rw; b; rw; b.}) to obtain optimized AIGs. % as much as possible. % After logic synthesis, the various SAT instances follow the similar distribution (see Fig.~\ref{FIG:syn}).  

% We further quantify the degree of uniformity of AIG distribution by introducing two measurements: the balance ratio (BR)~\cite{walker1976locally} and the logic level (Level). The balance ratio (BR) is defined as the average ratio of larger fanin region size to smaller fanin region size for each two-fanin gate, i.e. AND gate in AIG, which can reflect the balance degree of the binary fanin regions. A BR value closer to 1 indicates more balanced fanin regions of the gate. Logical level (Level) in the number of logic levels in a circuit, and a smaller number of logical levels indicates a more evenly distributed arrangement of the logical units. As can be observed from the Tab.~\ref{TAB:BRLevel}, the optimized AIGs typically have BR values that are closer to 1 and a smaller number of logical levels compared with those of the original AIGs, showing that the AIGs after optimization are more uniformly distributed. 

\begin{table}[t!]
\centering

\caption{The balance ratio and logic level before and after EDA opt. (Avg. $\pm$ Std.)} \label{TAB:BRLevel}
\resizebox{\linewidth}{!}{
\begin{tabular}{@{}l|ll|ll|ll@{}}
\toprule
                & \multicolumn{2}{c|}{Graph Coloring} & \multicolumn{2}{c|}{Random k-SAT} & \multicolumn{2}{c}{k-Clique} \\ 
                & BR               & Level           & BR             & Level           & BR           & Level         \\ \midrule
Before EDA opt. & $19.67 \pm 10.38$      & $45.71 \pm 7.04$      & $9.21 \pm 1.46$      & $67.58 \pm 34.34$     & $29.83 \pm 15.14$  & $106.75 \pm 44.00$  \\
After EDA opt.  & $1.16 \pm 0.09 $       & $14.15 \pm 0.99$      & $1.50 \pm 0.14$      & $12.40 \pm 0.96$      & $1.21 \pm 0.08$    & $13.29 \pm 0.81$    \\ \bottomrule
\end{tabular}}
\end{table}

\subsection{Other Quantitative Analysis}
Beside the balance ratio (BR) we present in the main context, we also evaluate the number of logic level ((Level), which indicates the depth of the circuits.  A smaller number of logical levels means a more evenly distributed arrangement of the logical units. As can be observed from the Tab.~\ref{TAB:BRLevel}, the optimized AIGs typically have BR values that are closer to 1 and a smaller number of logical levels compared with those of the original AIGs, showing that the distribution diversity of AIGs after optimization is reduced.

\begin{table}[t!]
\caption{The Error between Logic Simulation and Enumeration.}\label{tab:diff}
\centering
\begin{tabular}{@{}lll@{}}
\toprule
\# Samples & Difference & Error Rate \\ \midrule
100k       & 0.0007     & 1.75\%     \\
10K        & 0.0019     & 4.75\%     \\
1K         & 0.0144     & 36.00\%    \\
0.1K       & 0.1037     & 259.25\%   \\ \bottomrule
\end{tabular}
\end{table}

\section{Dataset Construction by Logic Simulation}\label{appendix:simulation}

% {
% \color{blue}
The constructed training dataset $\mathcal{D}$ consists of tuples of $(\mathcal{G}^{(i)}, \mathbf{m}^{(i)}, {\hat{\bm{\theta}}}^{(i)})$, where $\mathcal{G}^{(i)}$ is a Boolean circuit, $\mathbf{m}^{(i)}$ is a conditional mask and ${\hat{\bm{\theta}}}^{(i)}$ is the simulated probabilities for every node in the Boolean circuit. 
% % In practice, we also include training samples where we consider $y\!=\!0$ when generating the mask $\mathbf{m}$. 
% Please refer to Appendix~\ref{appendix:simulation} for more details about training dataset construction.}

In the logic simulation, we aim at estimating the probability of a node being logic `1', which is used as a supervision signal in the following experiments. Specifically, the probability is estimated by counting the number of times the value of a gate becomes logic `1' when feeding N random assignments to the circuit.  For example, if a gate becomes logic 1 for 1,000 times under 10,000 random patterns, then the supervision of this gate will be a real value 1,000/10,000=0.1, which is the estimated probability of this gate being logic `1'. 

Empirically, we apply $15$k random patterns to each AIG to construct the training data. Given a conditional mask $\mathbf{m}$, we only count the random patterns that fulfill the condition. A tiny example is shown in Figure~\ref{FIG:mask}. When we mask the PO as logic `1', the simulated probability of nodes will be changed accordingly.

\begin{figure}[t!]
	\centering
	\includegraphics[width=0.8 \linewidth]{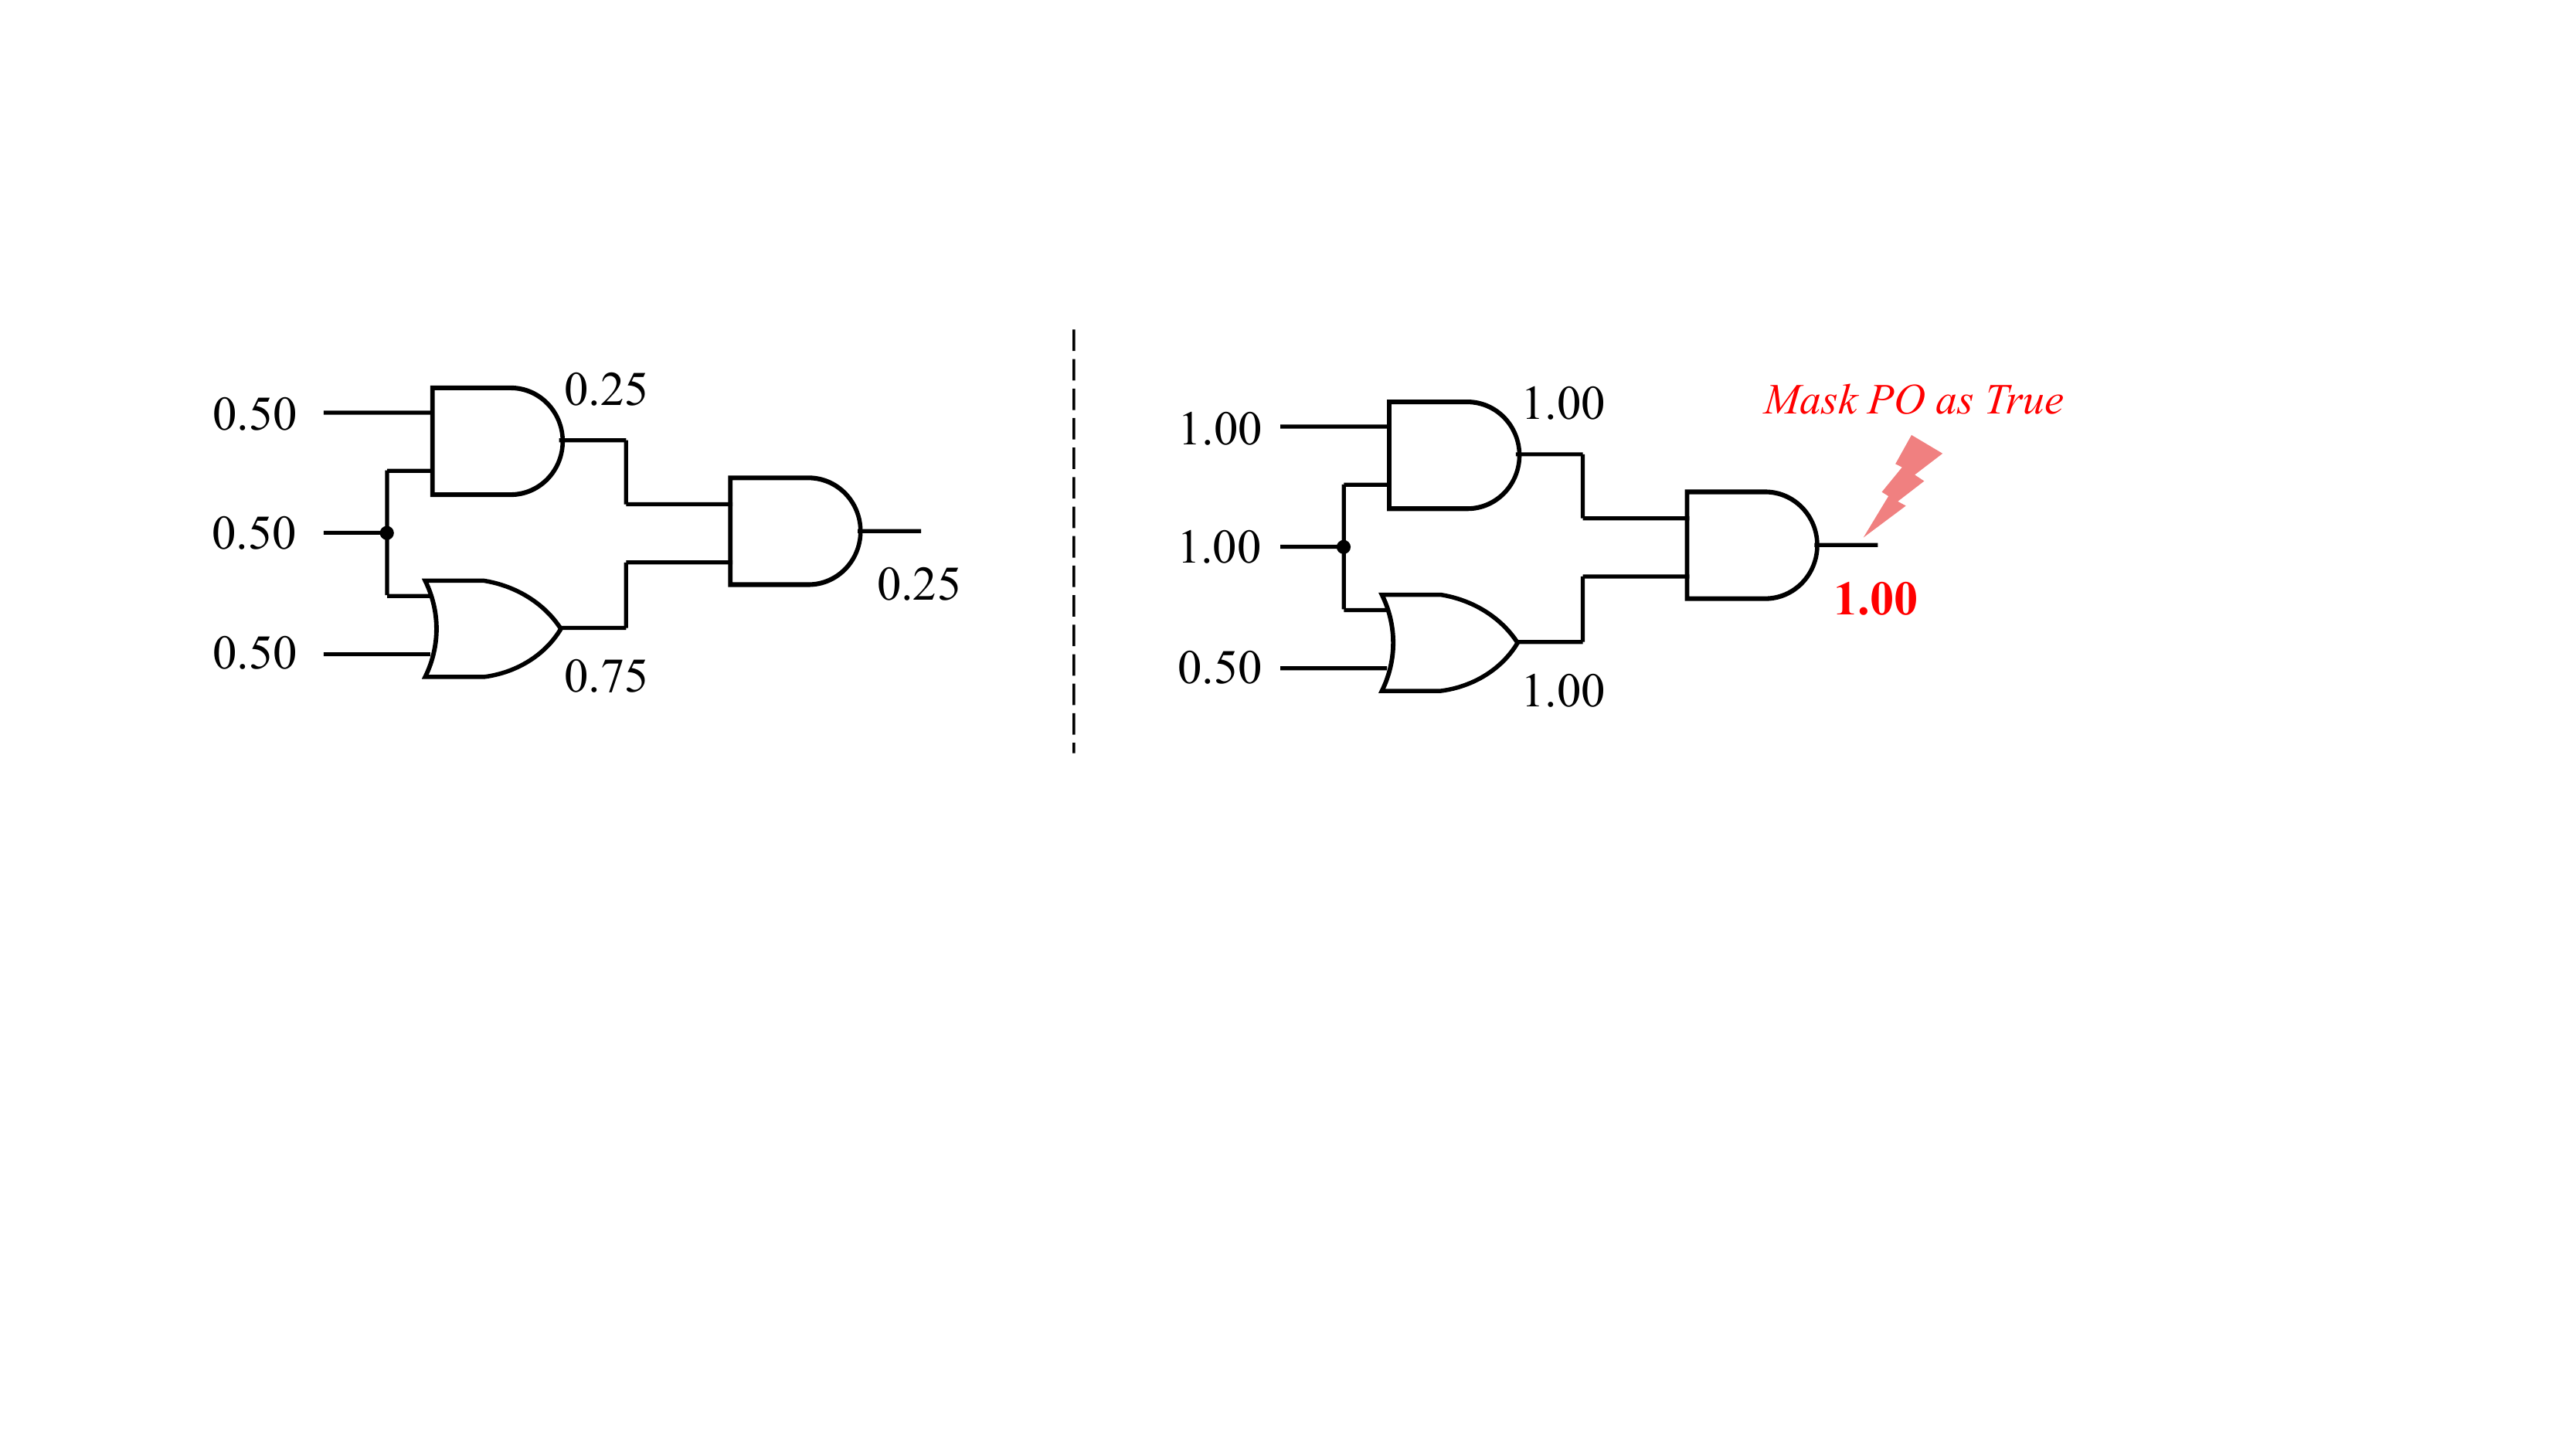}
	\caption{An example of logic simulation w/ and w/o mask.}
	\label{FIG:mask}
\end{figure}

In the previous end-to-end solutions~\cite{selsam2018learning,amizadeh2018learning}, a classical SAT solver is used to offer single-bit of supervision (SAT/UNSAT)~\cite{selsam2018learning}, or exclude unsatisfiable circuits from datasets~\cite{amizadeh2018learning}. Since the classical SAT solver is based on some hand-crafted searching heuristic, tens of thousands of  backtracking / branching are required to obtain the final satisfying solutions or give the unsatisfying certificates. On the other hands, the random simulation does not require any specialized designs, but a random input generator. Moreover, the logic simulation can be accelerated using parallelization algorithms and hardware (e.g., GPUs). Consequently, the cost of our logic simulation is on par with those of other learning-based SAT solving algorithms. For larger problems, an alternative is to first use an efficient “all solutions SAT solvers” to obtain all possible satisfying solutions, and then estimate the supervision signal $\hat{\theta}_i$ from these assignments. 

Similarly to \cite{li2021representation}, we observe that by applying $15$k random patterns to each AIG, we can achieve a balance between training efficiency and the quality of learning. 
We experiment with the numbers of samples ranging from 100 to 100k on the SR(20) training dataset (Table~\ref{tab:diff}). The results show that the performance stopped increasing after the number of samples reaching 10k. Note that for smaller SAT problems, we randomly generate samples without considering the repetitions. For exampple, we enumerate all possible assignments for an SR(20) instance and get the overall logic-1 probability as the ground truth. Then, we perform the logic simulation with 100K, 10K, 1K, and 0.1K samples. The table below shows the average difference between simulated logic-1 probability and ground truth. Since the final training loss of our model is about 0.04, the error caused by logic simulation with 10K samples is only 4.75\%. Therefore, we believe that simulating with 10K samples offers a good trade-off between simulation runtime and error. For the feasibility of covering enough satisfiable solutions, in our case, since the training dataset SR(3)-SR(10) is rather small, it is very likely that logic simulation with 10k patterns can cover enough satisfiable solutions for estimating. % For larger problems, a practical way is to first use an efficient “all solutions SAT solvers”  to obtain all possible satisfying solutions, and then estimate the supervision signal $\hat{\theta}_i$ from these assignments.

% \paragraph{Comparison with other training objectives.} In the previous end-to-end solutions~\cite{selsam2018learning,amizadeh2018learning}, the supervision for SAT problems is either weak or non-existent. In particular, NeuroSAT~\cite{selsam2018learning} leverages single-bit of supervision, i.e., whether the problem is satisfied or not, while CircuitSAT~\cite{amizadeh2018learning} only includes SAT problems into the training data, and trains the model in the unsupervised manner. Although both approaches can obtain the assignments if Boolean functions are satisfied, they do not explicitly take the assignments as the supervision into account during model training.

\section{Polarity Prototypes}\label{appendix:pp}

\subsection{Polarity Prototypes as Latent Space Regularization}
We interpret the polarity prototypes as one of latent space regularization techniques.  
Incorporating regularized structure into latent space is preferred in many scenarios, such as data generation~\cite{hadjeres2017glsr, kingma2013auto, shen2020interpreting}, unsupervised domain adoption~\cite{kang2019contrastive}, and few-show learning~\cite{snell2017prototypical}. In general, strategies belonging to this class make use of additional constraints imposed on the latent vectors, effectively reducing the extent of space each of them can occupy~\cite{barbato2021latent}. In this paper, we introduce two polarity prototypes with specific physical meanings (logic `$1$' or logic `$0$') into latent space, and facilitate learning a continuous and compact hidden space with good \textit{interpretability} of logic values. More importantly, with polarity-regularized embedding space, we can manipulate the states of nodes and thus do the conditional solution sampling.

\subsection{Learnable Polarity Prototypes}\label{appendix:learnable_prototypes}

Similar to learnable tokens in the Transformer-based models~\cite{dosovitskiy2021an, he2021masked, devlin2018bert}, we can randomly initialize two polarity prototypes and make them learnable along with the model parameters by back-propagation. By this way, the polarity prototypes can be discovered by the model automatically. In this subsection, we train another same DeepSAT model besides learnable polarity prototype and compare with the default setting (non-learnable polarity prototypes) under same training iterations. As a result, the model with learnable setting has PE = $0.1107$, which under-performs than the original DeepSAT model with fixed polarity prototypes (PE = $0.0648$). Therefore, we use the fixed polarity prototypes in our experiments.

\section{Solution Sampling Scheme}\label{appendix:infer}

In this section, we provide more details of our proposed solution sampling scheme. The pseudo-code is provided in Algorithm~\ref{algo:infer}. 

To sample solutions from the well-trained conditional model, we iteratively select the undetermined PI with the highest \textit{confidence} values predicted by the model, i.e., the PI with probability prediction closest to $0$ or $1$. Specifically, given an SAT instance $\mathcal{G}$ with $I$ variables, we conduct the following \textit{auto-regressive} procedure: 
\begin{enumerate}
    \item We mask PO as logic `1', and generate the corresponding mask vector $\mathbf{m}_0$.
    \item At $t$ iteration, we pass $(\mathcal{G},\mathbf{m}_{t})$ to well-trained DeepSAT model to estimate the simulated probability of all un-masked PIs. The PI with the highest confidence is selected and masked as logic `0' if the prediction is smaller than 0.5, otherwise logic `1'. According to the selected PI and its masked value, a new mask $\mathbf{m}_{t+1}$ is generated.
    \item Repeat the second step until all PIs have been masked ($I$ iterations in total). 
\end{enumerate}

To explore more possible assignments to satisfy the SAT instance, we also develop a simple \textit{flipping}-based strategy (line 17 - line 27 in Alg.~\ref{algo:infer}) to sample more solutions from the conditional model ($(I+1)$ solutions in the worst case). To be specific, during the initial solution sampling step, we record the masking order in the iteratively solving procedure as $\mathbf{O} = \{ o_1, o_2, …, o_n\}$. For the round $r$, where $r = 1, 2, …, n$, we modify the initial mask $\mathbf{m}_0^{r}$ as Eq.~\ref{eq:bitflipping}, where flip the $r^{th}$ approximated assignment and keep the former assignment as the initial mask $\mathbf{m}_0^r$ to estimate another possible solution. 

\begin{equation}
    m_{O_i} =\left\{
    \begin{array}{lcl}
        x_{O_i}^{*}       &      & i < r \\
        \neg x_{O_i}^{*}       &      & i = r \\
        0       &      & i > r
    \end{array}
    \right.
    \label{eq:bitflipping}
\end{equation}

For example, if we get the initial solution $\mathbf{x}^{*} = \{0, 0, 0\}$ for a three variable SAT instance and the iterative order is $\mathbf{O} = \{v_3, v_2, v_1\}$. For the round $r=1$, the initial mask should be $\mathbf{m}_0^1 = \{ m_{PO} = 1, m_{O_r} = \neg x_{O_r}^{*}\}$, i.e., $\mathbf{m}_0^1 = \{ m_{PO} = 1, m_{v_3} = 1\}$. For the round $r=2$, the initial mask should be $\mathbf{m}_0^2 = \{ m_{PO} = 1, m_{v_3} = 0, m_{v_2} = 1\}$. 
The above re-sampling procedure is executed until finding a satisfying solution or exceeding round $n$. %The bit flipping procedure is different from the naïve searching or heuristic searching, where our procedure only performs up to $n$ rounds. 

\begin{algorithm}[t]
\caption{Conditional Inference with Backtracking}
\label{algo:infer}
\KwIn{The problem instance in AIG format $\mathcal{G}$. The number of variables $\text{\#}var$. The trained model $\text{DeepSAT}$.}
\KwOut{Return the satisfiable assignment (for predicted SAT instance) or empty $\varnothing$ (for predicted unknown instance)}
    \tcc{Iterative solving function}
    \SetKwFunction{FMain}{IterativeSolve}
    \SetKwProg{Fn}{Function}{:}{}
    \Fn{\FMain{$\mathcal{G}, \text{DeepSAT}, agn, \text{\#}var$}} {
        $NoAgned = \text{\#}var - (agn == 0)$ ; \\
        $\mathbf{O} = \varnothing$ ; \\
        \For{$it \leftarrow NoAgned$ \ \KwTo \  $\text{\#}var$} {
            $\mathbf{m} = \text{obtainMask}(agn)$ ; \tcp{Generate mask}
            $\mathbf{V} = \text{DeepSAT}(\mathcal{G}, \mathbf{m})$; \\
            $idx = \text{findMostConfidentDecision}(\mathbf{V}, agn)$ ; \\
            $agn[idx] = (\mathbf{V} < 0.5) \ ? \ -1: 1$ ; \\
            $\mathbf{O}\text{.append}(idx)$ ; \tcp{Save decision order}
        }
        \Return $(agn, \mathbf{O})$ ; \\
    }
    
    \tcc{Initial solving assumption}
    $\mathbf{x}^{*} = [0] * \text{\#}var$ ; \\
    $\mathbf{x}^{*}, \mathbf{O} = \text{IterativeSolve}(\mathcal{G}, \text{DeepSAT}, \mathbf{x}^{*}, \text{\#}var)$ ; \\
    \If{$\text{VerifySolution}(\mathcal{G}, \mathbf{x}^{*})$} {
        \Return $\mathbf{x}^{*}$ ; \\
    }
    
    \tcc{\textit{Flipping}-based strategy with $\mathbf{O}$}
    \For{$i \leftarrow 0$ \ \KwTo \  $len(agn)$} {
        $agn = [0] * \text{\#}var$ ; \\
        \For{$j \leftarrow 0$ \KwTo $i$} {
            $agn[\mathbf{O}[j]] = \mathbf{x}^{*}[j]$ ; \tcp{Pre-assign the variables}
        }
        $agn[\mathbf{O}[i]] = (agn[\mathbf{O}[i]] == 1) \ ? \ -1 : \ 1$ ; \tcp{Flip one assigned variables}
        $agn, \_ = \text{IterativeSolve}(\mathcal{G}, \text{DeepSAT}, agn, \text{\#}var)$ ; \tcp{Try another assumption}
        \If{$\text{VerifySolution}(\mathcal{G}, agn)$} {
            \Return $agn$ ; \\
        }
    }
    \Return $\varnothing$ ; \tcp{Fail to find assignment, mark the instance as unknown}
\end{algorithm}

\section{Implementation Details and Comparison to Related Models}\label{appendix:baselines}

\subsection{Different Circuit formats}\label{appendix:circuit}
\begin{figure}[t!]
	\centering
	\includegraphics[width=0.7\linewidth]{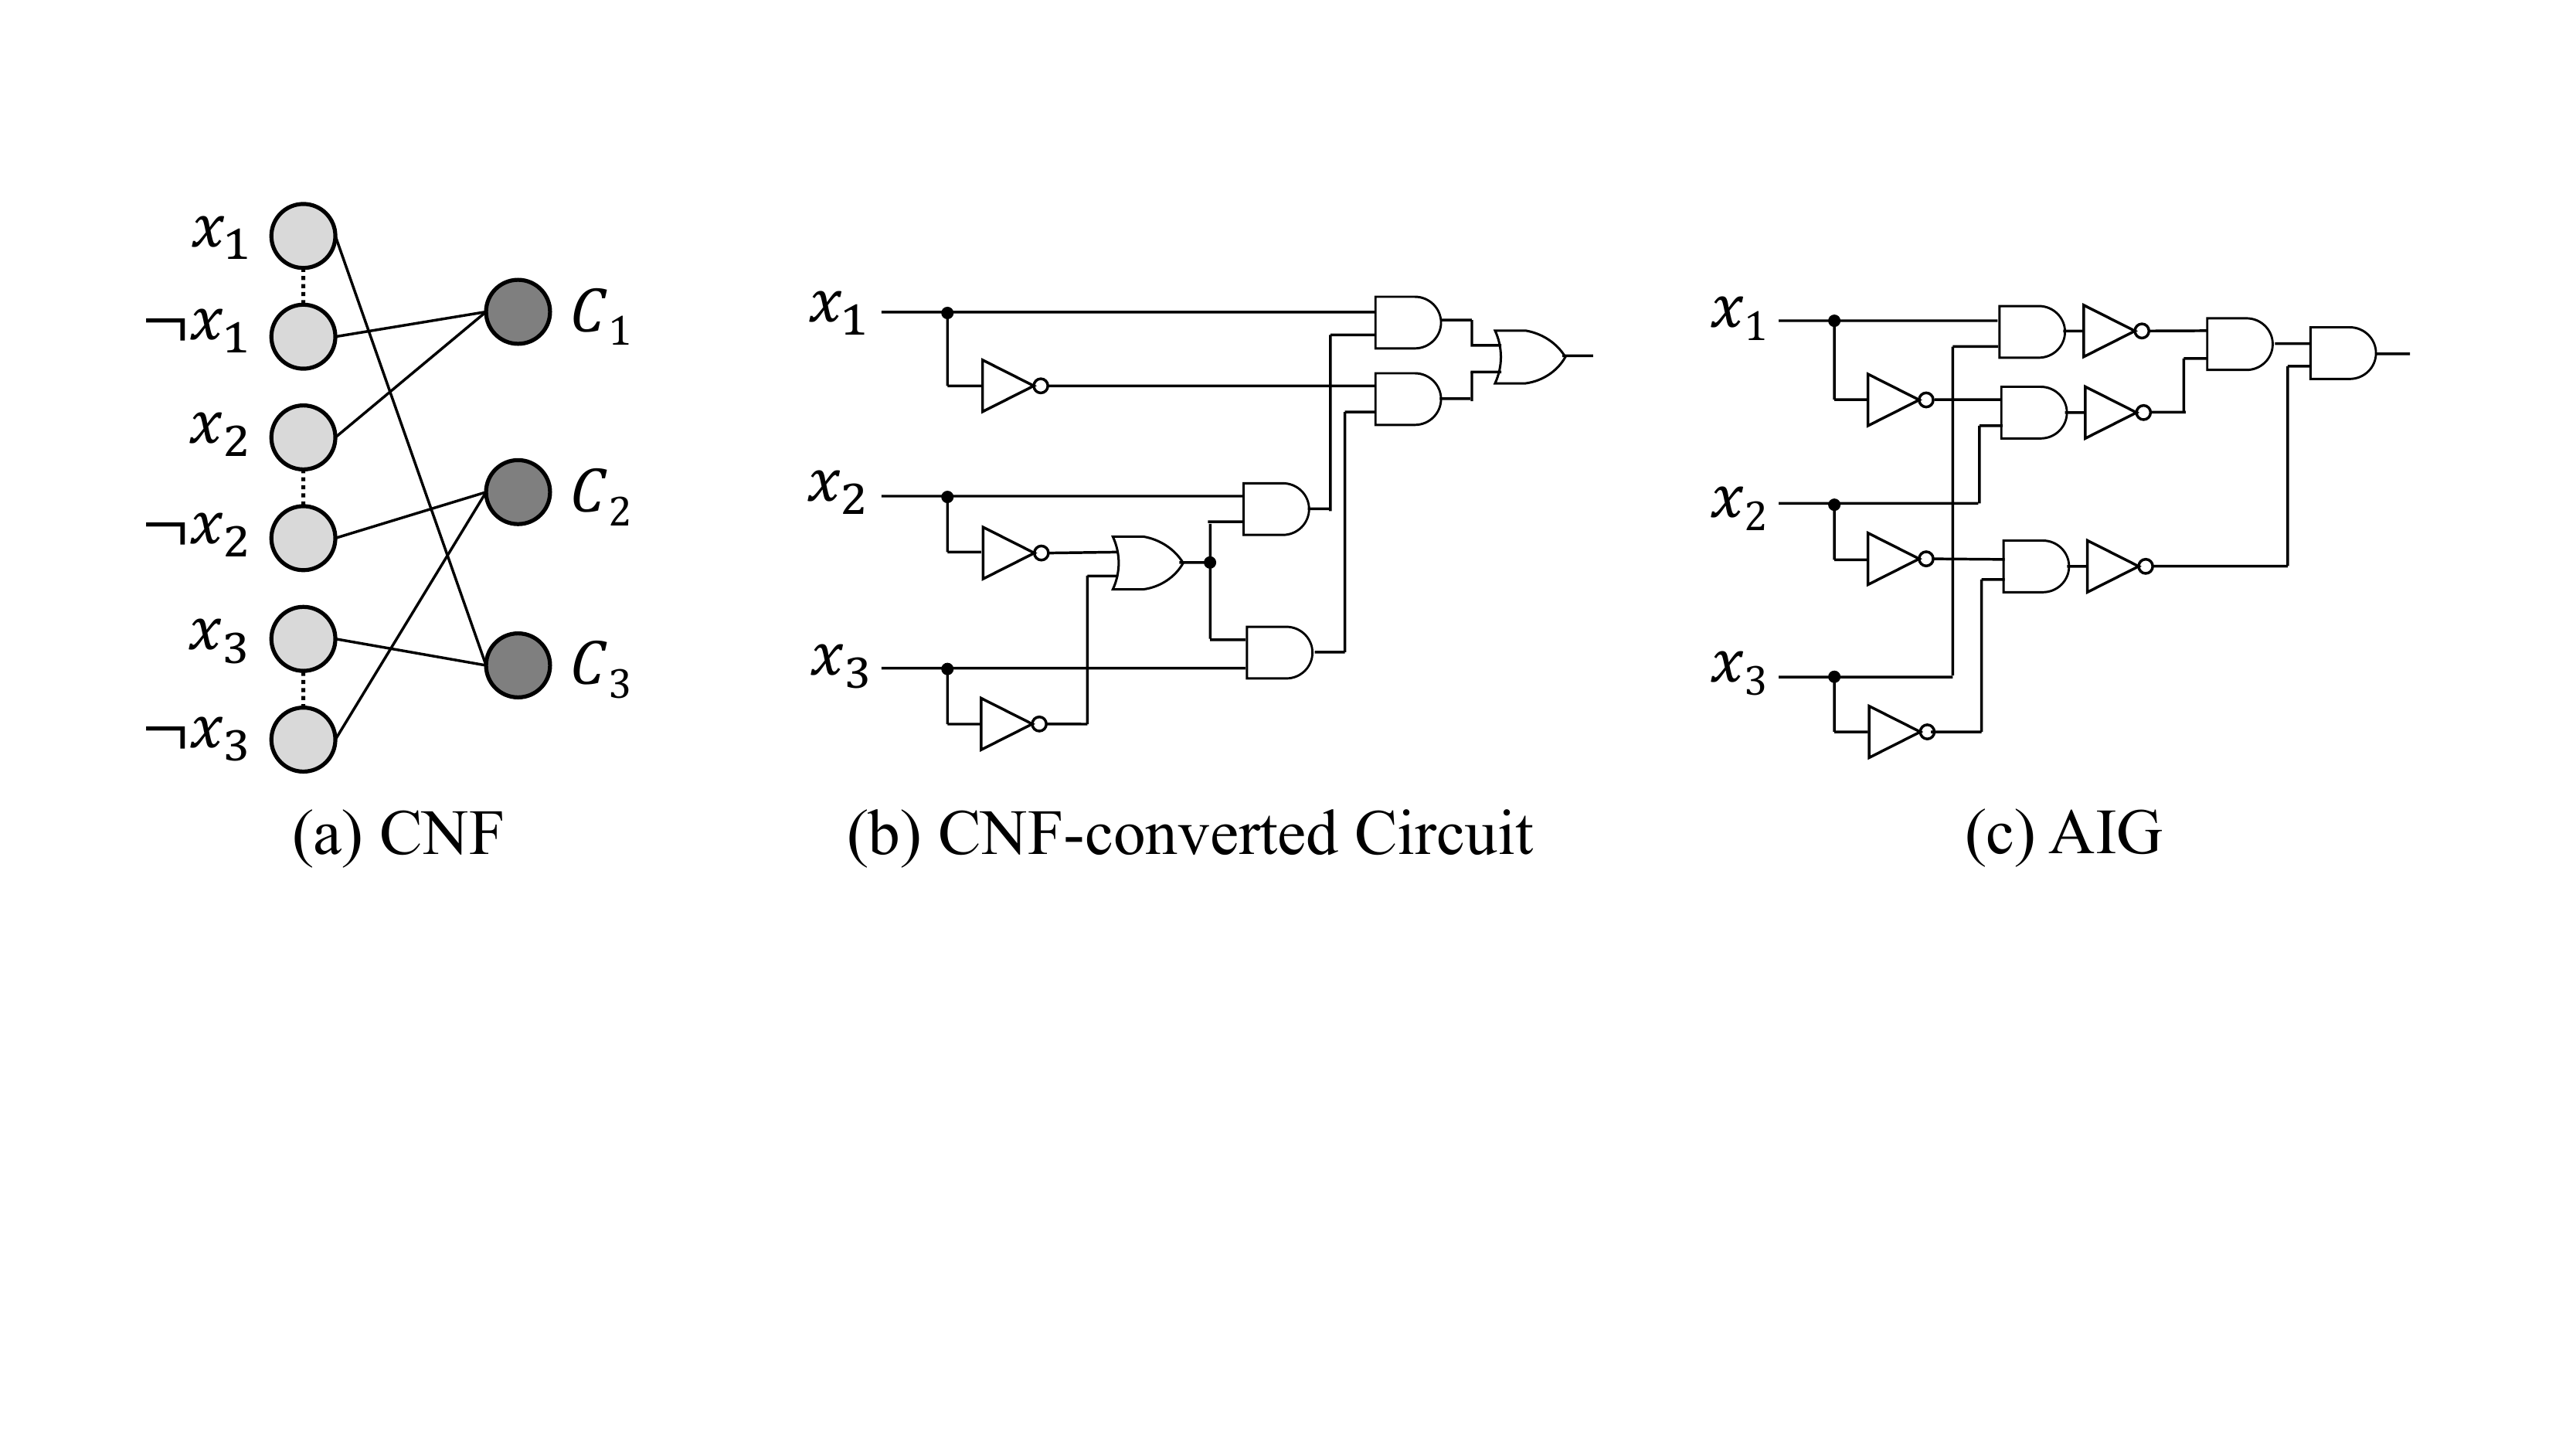}
	\caption{Three graph representations of the Boolean formula in Equation~\ref{eq:sat_example}.}
	\label{FIG:graphRep}
\end{figure}

NeuroSAT consumes CNF as a bipartite graph, while DG-DAGRNN and DeepSAT can process various circuit formats. Here we give an example of SAT instances, and visualize it under different circuit formats in  Figure~\ref{FIG:graphRep}. The example we use is Equation~\ref{eq:sat_example} in the CNF format, which consists of 3 variables.  

% Equation~\ref{eq:sat_example} and Figure~\ref{FIG:graphRep}.

\begin{equation}
    \phi := (\neg x_1 \lor x_2) \land (\neg x_2 \lor \neg x_3) \land (x_1 \lor x_3)
    \label{eq:sat_example}
\end{equation}

\subsection{Implementation Details of DeepSAT}
\begin{table}[!t]
\caption{The training and model setting of default DeepSAT} \label{TAB:AP:Setting}
\centering
\begin{tabular}{@{}lll@{}}
\toprule
                          & Configuration           & Value                 \\ \midrule
\multirow{5}{*}{Training} & Optimizer               & Adam                  \\
                          & Learning rate           & 1e-4                  \\
                          & Weight decay            & 1e-10                 \\
                          & Training epochs         & 20                    \\
                          & Batch size              & 64                    \\ \midrule
\multirow{4}{*}{Model}    & Hidden vector dimension & 64                    \\
                          & Aggregator              & Attention             \\
                          & Update function         & GRU                   \\
                          & Regressor               & 3-layer MLP with ReLU \\ \bottomrule
\end{tabular}
\end{table}

DeepSAT consists of one forward propagation layer and one reverse propagation layer. In particular, we use a single-layer GRU and a attention-based aggregation function to instantiate each propagation layer. The forward propagation layer and reverse propagation layer do not share the parameters. The dimension of node hidden states is set as $64$. The regressor is a 3-layer MLP with hidden dimension $64$. 
We train DeepSAT for $60$ epochs with batch-size $128$ on 4 Nvidia V100 GPUs. The Adam optimizer~\cite{kingma2014adam} is adopted with the learning rate $10^{-4}$ and weight decay $10^{-10}$. We use the topological batching technique introduced in \cite{thost2021directed} to accelerate the training. The details of the model setting and training setting are listed in Tab.~\ref{TAB:AP:Setting}
% {\color{red}We provide the full details of model architecture and the ablation study of hyper-parameters in Appendix~\ref{appendix:model}. }

\subsection{Implementation Details of NeuroSAT}
NeuroSAT supports the instance in CNF format. We reproduce the NeuroSAT based on the original configurations. The message-passing is performed for $10$ iterations between literals and clauses during training. The dimension of node hidden states is $128$. 

\subsection{Implementation Details of DG-DAGRNN}
DG-DAGRNN is a GNN model specialized for Circuit-SAT problems. 
Following the the original paper, we set the number of node hidden states is $100$. We also adjust temperature $\tau$ in evaluator network dynamically as $\tau = t^{-0.4}$, where $t$ is the number of training epochs. The $k$ in loss function is set $10$ in the following experiment. Besides, we set the number of GNN iterations as $10$. 

Besides the model configuration in~\cite{amizadeh2018learning}, we also provide the modified configuration to further improve the model performance. 
1) Since the CNF is converted into a circuit based on Cube and Conquer paradigm~\cite{heule2011cube}, the number of fan-in wires for different gates is not fixed. The original aggregation function in GNN sums up all messages from predecessors without considering the various number of fan-in wires. We replace the original aggregation with an attention-based aggregation function~\cite{li2021representation} to calculate the weighted sum. 
2) The original DG-DAGRNN includes a linear projection to project the hidden state into lower dimension vectors and feedback as the next layer inputs. The information about gate type loses after multiple message-passing rounds. We remove the linear projection and directly feedback the concatenation of hidden state and one-hot encoded gate type into next layer propagation. 
3) The SAT instance in the original training dataset consists of a large number of clauses. Usually, there are only $1$ or $2$ out of $2^{n}$ satisfiable assignment for a SR($n$) instance. Find an assignment to satisfy such instance is extremely difficult. We augment the training dataset with many simple instances by removing the clauses from the difficulty instances.

We try to reproduce DG-DAGRNN (including the original configuration and our modified configuration described above) and also apply the same EDA optimizations to it, as the official code of DG-DAGRNN remains publicly unavailable up to now. In order to test the correctness of our implementation, we try our re-implementation of DG-DAGRNN on SR($3$) problems and train for $200$ epochs. As the instances in the training dataset are easily satisfied by random guessed assignment, the initial testing accuracy is $33\%$. After training for the first $86$ epochs, the testing accuracy improves only $1\%$. The model converges after $100$ epochs and only achieves $44\%$ testing accuracy. Although we explore the other configurations with different $k$ values in the loss function ($k=0.1, 1, 5, 10$), the model still converges slowly and only improves a little testing accuracy. Unfortunately, when we train the model on the same dataset in DeepSAT (Section~\ref{sec:exp}), with all the efforts, we still fail to train DG-DAGRNN to converge.

We attribute the difficulty of training DG-DAGRNN to its vulnerability to training crash. On the one hand, DG-DARGNN employs a soft-evaluator as the reward network and is a variant of Policy Gradient method during training. As we observe empirically, the training is sensitive to several hyper-parameters and is extremely difficult to optimize even we follow the same setting described in the original paper. On the other hand, increasing the number of logical levels would result in a large stack of smoothed max and min functions in DG-DAGRNN. Consequently, the gradient tends to vanish and thus the training tends to fail. Moreover, even though we cannot reproduce DG-DAGRNN, the results DeepSAT obtains is still better than the ones reported in the original paper.

Note that we will add DG-DAGRNN as another baseline once the authors release the code.

\subsection{Comparison to Related Works}

We compare DeepSAT with NeuroSAT in the main text, and describe the reason why we do not consider DG-DAGRNN as the baseline above. Besides NeuroSAT and DG-DAGRNN, there are other existing end-to-end SAT solutions. We enumerate the published works here and elaborate the differences between these models and DeepSAT. In addition, we give the explanation why we consider NeuroSAT as the strong baseline in our experiments.

ContrastiveSAT~\cite{duan2022augment} studies contrastive learning on end-to-end SAT solvers. They demonstrate that using label-preserving augmentations of CNFs can learn a meaningful representation, which can achieve achieve comparable test accuracy to fully-supervised learning while using only $1\%$ of the labels for finetuning. The baseline is also NeuroSAT. The code of this work is not open-sourced and they only argue a similar performance of proposed method compared with NeuroSAT. In addition, they follow a unsupervised setting, which is differs from ours. Thus, we do not consider ContrastiveSAT as another baseline.

\cite{yolcu2019learning, kurin2020can} use Reinforcement Learning to train branching heuristic in stochastic local search (SLS) solvers and conflict driven clause learning (CDCL) solvers. The input representation in these two works all follows the one used in NeuroSAT: a bipartite graph representation defined by CNF. More importantly, the design principle of graph neural networks is the same with NeuroSAT, where the message passing is iteratively conducted between literals and clauses. These two works are learning-aided SAT solvers, and in the original works the baselines are classical SAT solvers. Therefore, we do not consider them as the baselines for comparison. Note that the proposed DeepSAT has the potential to aid the conventional Circuit-SAT solvers, and we plan to explore this direction in the future work.

% For QuerySAT, we will take it as another baseline in the next version of the manuscript and make a more detailed discussion with QuerySAT in related work. 

NLocalSAT~\cite{zhang2021nlocalsat} is a learning-aided SAT solver, which boosts the stochastic local search (SLS) solvers by initializing the assignments, which is compared with classical SLS solvers such as CCAnr and YalSAT. Though NLocalSAT can also be evaluated as an end-to-end SAT solver, the model structure of NLocalSAT is almost the same as NeuroSAT, expect the authors modify the learning objective. Hence, we compare our model with NeuroSAT directly.

\section{Discussion on evaluation metric for end-to-end SAT solvers}\label{appendix:metric}
Since the proposed DeepSAT is an incomplete solver, it predicts a problem as SAT if and only if it finds a satisfying assignment, otherwise returns UNKNOWN. To this end, if we evaluate DeepSAT on both SAT and UNSAT instances,  the false positive rate (FP) will be 0 because the UNSAT ones would never be predicted as SAT by DeepSAT. Moreover, we focus on generating a solution for SAT instead of the binary SAT/UNSAT prediction problem, since the latter is less attractive unless a satisfying assignment can be given for every instance that is predicted as SAT. Therefore, we only consider testing on satisfiable instances. Note that testing only on satisfiable instances is also adopted in DG-DAGNN.

% From DG-DAGRNN: Similar to Selsam et al. (2018), we could also approach the Circuit-SAT problem from two different angles: (1) predicting the circuit satisﬁability problem as a binary classiﬁcation problem, and (2) solving the Circuit-SAT problem directly by generating a solution if the input circuit is indeed SAT. In Selsam et al. (2018), solving the former is the prerequisite for solving the latter. However, that is not the case in our proposed model and since we are interested to actually solve the SAT problems, we do not focus on the binary classiﬁcation problem. Nevertheless, our model can be easily adapted for SAT classiﬁcation, as illustrated in Appendix A.

\section{Additional Analysis}\label{appendix:additional}
In this section, we conduct ablation studies to investigate the effectiveness of our proposed methods. To enable a fair comparison, all models are trained for 10 epochs. Beside the evaluation metric \textit{Problem Solved} defined in Section~\ref{Sec:Exp:Imp}, we also report \textit{Prediction Error} (PE), the least absolute error between the prediction and the supervision label. PE can be treated as the loss of models during training and validation, reflecting how well the model fits into the datasets.
In general, PE has a strong correlation with the metric \textit{Problem Solved}. The smaller PE is, the higher \textit{Problem Solved} model can achieve. 
% Consequently, we use PE to evaluate the capability of conditional modeling under different settings.
Besides, we construct a validation SAT dataset with 100 SAT instances. %and  evaluate the performance on the dataset.

\subsection{Solution Sampling Scheme}\label{appendix:sample}
The number of re-sampling varies for different problems. We show the statistics of the number of sampling solutions for solving 100 SR(10) problems (Table~\ref{tab:sr10}) and 100 SR(20) problems (Table~\ref{tab:sr20}). As can be observed, DeepSAT samples 1.6 solutions on average for SR(10) and terminates when the latest sampled solutions are satisfying. In terms of the number of iterations, the results are still better than the baselines. The result on 100 SR(20) shows the same tendency.

\begin{table}[t!]
\caption{The number of problems solved v.s. the number of sampled solutions for SR(10)}\label{tab:sr10}
\centering
\begin{tabular}{@{}cccccccccccc@{}}
\toprule
\# Sample Solutions & 1  & 2 & 3  & 4 & 5 & 6 & 7 & 8 & 9 & 10 & 11 \\ \midrule
\# Problem Solved   & 72 & 8 & 11 & 1 & 2 & 2 & 1 & 0 & 1 & 0  & 0  \\ \bottomrule
\end{tabular}
\end{table}

\begin{table}[t!]
\caption{The number of problems solved v.s. the number of sampled solutions for SR(20)}\label{tab:sr20}
\centering
\resizebox{\linewidth}{!}{
\begin{tabular}{@{}ccccccccccccllllllllll@{}}
\toprule
\# Sample Solutions & 1  & 2  & 3  & 4 & 5 & 6 & 7 & 8 & 9 & 10 & 11 & 12 & 13 & 14 & 15 & 16 & 17 & 18 & 19 & 20 & 21 \\ \midrule
\# Problem Solved   & 66 & 5 & 4 & 2 & 0 & 2 & 1 & 0 & 1 & 2  & 0  & 0  & 0  & 0  & 1  & 1  & 0  & 0  & 0  & 0  & 0  \\ \bottomrule
\end{tabular}}
\end{table}
Please note that even though the DeepSAT produces I+1 solutions in the worst case (`I=number of vars`), in most cases, the proposed method can generate satisfying assignments in the first few sampling rounds.

Furthermore, to explore the effectiveness of our proposed solution sampling scheme in Section~\ref{subsec:sat-infer}, we design other three simplified sampling schemes and use 100 SR($10$) problems to evaluate them. %We use 1000 SR10 problems in each setting for a fair comparison among these three inference scheme. 
In the first sampling scheme, we only mask the PO and use DeepSAT to get the probabilities of sat assignments on PIs. By setting the threshold at 0.5, we obtained 4\% accuracy under this setting. In the second inference setting, we again mask the PO, but use DeepSAT iteratively to achieve the SAT assignment on each PIs one by one. During each iteration, we choose the PI with most uncertain probability (i.e., PI with probability around 0.5) to be masked. We obtained only 1\% accuracy under this setting. In the third inference setting, we again mask the PO and use DeepSAT iteratively to achieve the SAT assignment on each PIs one by one. But during each iteration, we choose the PI with most certain probability i.e., either close to 1 or close to 0, to be masked. We obtained 70\% accuracy under this setting.

To sum up, the proposed inference scheme outperforms other simplified sampling schemes. Note that in this work, we keep the solution sampling scheme as simple as possible. We expect designing more complex sampling designs to be able to further improve DeepSAT’s performance. For example, we can use Reinforcement Learning to train an agent to decide which PI to be masked during sampling. We leave it for future work.

\subsection{Effectiveness of Directed Acyclic GNNs}\label{appendix:gnn}
To verify the effectiveness of our DAG-based design in Section~\ref{subesec:task}, we compare the performance of \textit{Directed} GNN models and \textit{Undirected} GNN models. For the undirected GNN, we replace the forward and reverse propagation as two undirected propagation layers, where the propagation is conducted bidirectionally and simultaneously. Both  models are equipped with the attention-based aggregator~\cite{thost2021directed, velivckovic2018graph} as Equation~\ref{eq:attn}. The experimental results are shown in Table~\ref{TAB:AP:DAG}. The directed model with Attention aggregator shows PE = $0.0648$ and solves $64\%$ SAT problems. Not surprisingly, since the undirected model does not capture the relational bias in circuits, such a model performs poorly in representing circuits. In addition, the undirected model with the same aggregator almost solves no SAT problems because the model predicts the masked simulation probability quite inaccurate (PE = $0.4297$).

% To verify the effectiveness of our DAG-based design as Section~\ref{subesec:task}, we compare the performance of \textit{Directed} GNN models and \textit{Undirected} GNN models with four different aggregators. The experimental results are shown in Tab.~\ref{TAB:AP:DAG}. First, the attention-based aggregator~\cite{thost2021directed, velivckovic2018graph} as Eq.~\ref{eq:attn} has the lowest PE than the other three aggregators, including the convolutional sum (abbr. Conv. Sum)~\cite{selsam2018learning}, Gated Sum~\cite{zhang2019d} and DeepSet~\cite{amizadeh2018learning}. We suppose that the attention mechanism allocates a higher attention weight to these dominant node neighbors. Second, the average PE of the undirected model is about $6.50$ times larger than the directed model. Since the undirected model ignores the computational behavior with logic ordering, such a model is not skilled in representing circuits. 

% Not surprisingly, the trained undirected models almost solve no SAT problems because these models predict the masked simulation probability quite inaccurate (PE = $0.4297$ on average). Contrarily, the DAG-based models perform better, and the model with an attention-based aggregator shows the best result. 

\begin{table}[!t]
\caption{The comparison of directed and undirected model} \label{TAB:AP:DAG}
\centering
\begin{tabular}{@{}llcc@{}}
\toprule
Model                       & Aggregator         & Prediction Error     & Problem Solved \\ \midrule
\multirow{4}{*}{Undirected} & Conv. Sum          & 0.4296 & 1\%            \\
                            & DeepSet            & 0.4298 & 0\%            \\
                            & GatedSum           & 0.4299 & 0\%            \\
                            & \textbf{Attention} & 0.4297 & 1\%            \\ \midrule
\multirow{4}{*}{Directed}   & Conv. Sum          & 0.0669 & 33\%           \\
                            & DeepSet            & 0.0651 & 57\%           \\
                            & GatedSum           & 0.0675 & 35\%           \\
                            & \textbf{Attention} & 0.0648 & 64\%           \\ \bottomrule
\end{tabular}
\end{table}

\begin{figure}[t!]
	\centering
	\includegraphics[width=0.7\linewidth]{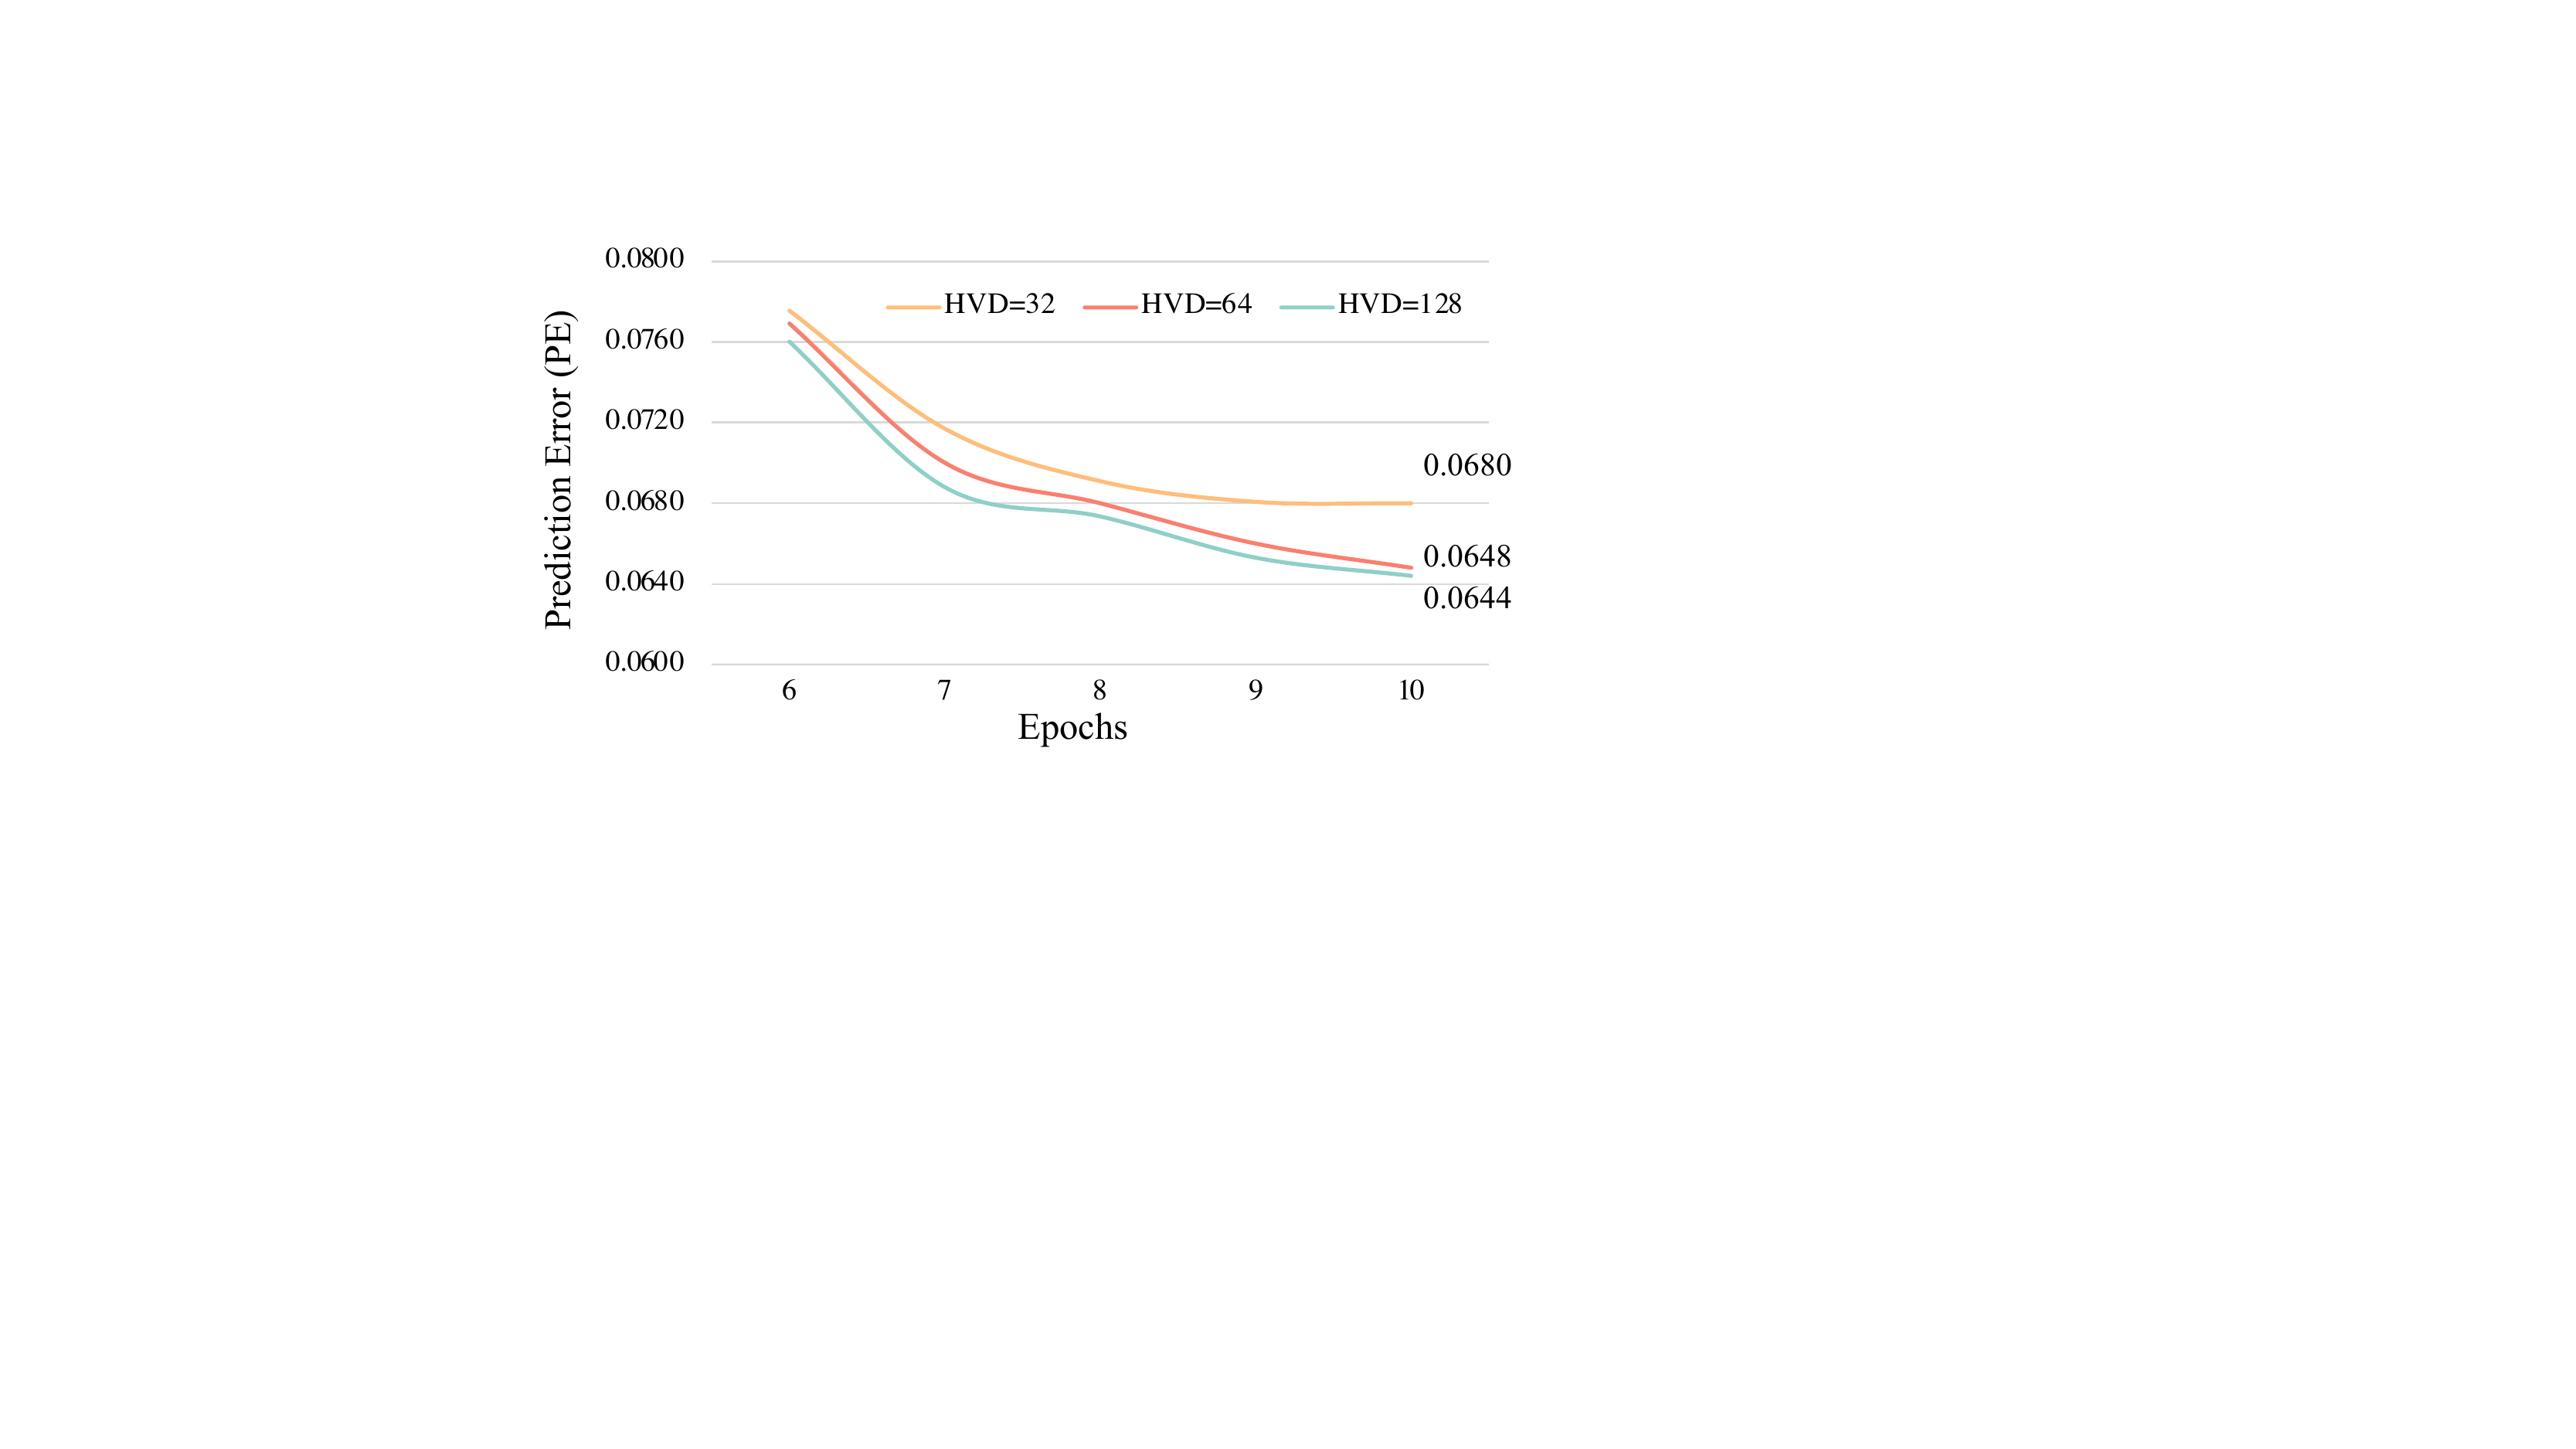}
	\vspace{-10pt}
	\caption{The comparison of models with different hidden vector dimension for prediction errors.}
	\label{FIG:AP:PE}
	\vspace{-15pt}
\end{figure}

\subsection{Different Aggregation Function} \label{appendix:Aggregation}
In order to demonstrate the effectiveness of aggregation function in Equation~\ref{eq:attn}, we compare Attention-based aggregation with other 3 different aggregator designs, which include representative works for DAG learning, i.e., Convolutional Sum (abbr. Conv. Sum)~\cite{selsam2018learning}, Gated Sum~\cite{zhang2019d} and DeepSet~\cite{amizadeh2018learning}. 
The attention-based aggregator has the lowest PE (PE = $0.0648$) than the other three aggregators, including the Conv. Sum (PE = $0.0669$), Gated Sum (PE = $0.0675$) and DeepSet (PE = $0.0651$) (see Tab.~\ref{TAB:AP:DAG}). We suspect that the superiority of the attention mechanism comes from its modeling capacity for logic computation. 
Specifically, when we do the logic computation in digital circuits, the controlling value of a logic gate determines the output of that gate. Therefore, controlling values are far more important than non-controlling values. To mimic this behaviour, the attention mechanism can learn to assign high weights for controlling inputs of gates and give less importance to the rest of the inputs.
allocates a higher attention weight to these dominant node neighbors. 
In summary, the DAG-based models with an attention-based aggregator achieves the best results, compared to other kinds of aggregation functions.

\subsection{Hidden Vector Dimension} \label{appendix:latentDim}
% the decreasing prediction error and increasing problem solved percentage indicate that the model has better representation ability. However, the model will cost much runtime with the more complex model structure. As we can see in the Improvement column, the problem solved percentage improves $42.22\%$ from $45\%$ to $64\%$ when we enlarge the latent vector dimension twice from $32$. However, such improvement only is $10.94\%$ while the dimension increases from $64$ to $128$.

We investigate the influence of the hidden vector dimension (HVD) by training three models with three different setting: HVD = $32$, $64$ and $128$, respectively. The prediction errors of various configurations in the last $5$ epochs are shown in Figure~\ref{FIG:AP:PE}. With the increasing hidden vector dimension, the prediction error decreases. Yet, we observe that with more training iterations, the performance gap between models with latent vector dimension as $64$ and $128$ becomes less significant. At training epochs $10$, the PE gap is only $0.0004$, about $0.62\%$ PE of the model with $64$ hidden vector dimension. Therefore, we set the latent vector dimension as $64$ in the experiments.

% \subsection{DeepSAT-Aided SAT Solver}

% This DeepSAT model is ready to be a pre-processing module for some heuristics-based SAT solver. For example, DeepSAT can give a promising initialization assignments for Random-Walk~\cite{yolcu2019learning}. Another work is~\cite{zhang2021nlocalsat}, in which the authors claim that NLocalSAT is the first work to combine Stochastic Local Search (SLS) with a NN model. However, ~\cite{yolcu2019learning} must be the first one.

% The core idea in~\cite{zhang2021nlocalsat} is to better initialize the assignments for SLS, while in~\cite{yolcu2019learning} is to better have a heuristics for selecting variables for bit flipping. I think DeepSAT can all be applied in these two cases.
